# Supplementary material for: Attacking Visual Language Grounding with Adversarial Examples: A Case Study on Neural Image Captioning
Source: arXiv:1712.02051 source file (2018-05-22)
Supplement: Supplementary file 1 [file supp_for_review.tex]

\documentclass[10pt,twocolumn,letterpaper]{article}

\usepackage{cvpr}
\usepackage{times}
\usepackage{epsfig}
\usepackage{booktabs}
\usepackage{graphicx}
\usepackage{algorithm}
\usepackage{tabulary}
\usepackage[noend]{algpseudocode}
\usepackage{subcaption}
\usepackage{paralist}
\makeatletter
\def\BState{\State\hskip-\ALG@thistlm}
\makeatother
\usepackage[page]{appendix}
\usepackage{comment}
\usepackage{amsmath}
\usepackage{amssymb}
\usepackage{mathtools}
\usepackage{bm} % bold math symbol

% Include other packages here, before hyperref.

% If you comment hyperref and then uncomment it, you should delete
% egpaper.aux before re-running latex.  (Or just hit 'q' on the first latex
% run, let it finish, and you should be clear).
\usepackage[pagebackref=true,breaklinks=true,letterpaper=true,colorlinks,bookmarks=false]{hyperref}
\urlstyle{same}
% \cvprfinalcopy % *** Uncomment this line for the final submission

 % *** Enter the CVPR Paper ID here

% Pages are numbered in submission mode, and unnumbered in camera-ready
\ifcvprfinal\pagestyle{empty}\fi

\makeatletter
\newcommand{\customlabel}[2]{%
   \protected@write \@auxout {}{\string \newlabel {#1}{{#2}{\thepage}{#2}{#1}{}} }%
   \hypertarget{#1}{#2}
}
\makeatother

\begin{document}

%%%%%%%%% TITLE
\title{Supplementary Materials of \\Show-and-Fool: Crafting Adversarial Examples for Neural Image Captioning }

\author{Hongge Chen\textsuperscript{1}\thanks{Hongge Chen and Huan Zhang contribute equally to this work.}\enskip, Huan Zhang\textsuperscript{2}\footnotemark[1]\enskip\thanks{Work done during internship at IBM T. J. Watson Research Center}\enskip, Pin-Yu Chen\textsuperscript{3}, Jinfeng Yi\textsuperscript{4}, Cho-Jui Hsieh\textsuperscript{2} \\
\textsuperscript{1}Massachusetts Institute of Technology, Cambridge, MA 02139\\
\textsuperscript{2}University of California Davis, Davis, CA 95616\\
\textsuperscript{3}IBM T.J. Watson Research Center, Yorktown Heights, NY, 10598\\
\textsuperscript{4}Tencent AI Lab, Bellevue, WA 98004\\
{\tt\small chenhg@mit.edu, ecezhang@ucdavis.edu,}\\ 
{\tt\small Pin-Yu.Chen@ibm.com, jinfengyi@tencent.com, chohsieh@ucdavis.edu}}

\maketitle
%\thispagestyle{empty}

%%%%%%%%% BODY TEXT
\setcounter{figure}{3}
\setcounter{table}{5}
\input{supp}
\clearpage
{\small
\bibliographystyle{ieee}
\bibliography{paperbib}
}
See the main text for Table \customlabel{tab:transfer}{5}, equation \customlabel{eq:softmaxloss}{7}, \customlabel{eq:general_loss}{3}, \customlabel{eq:logits loss}{11} and section \customlabel{subsec_transfer}{4.5}.
\end{document}
